# Supplementary material for: Random heterogeneity outperforms design in network synchronization
Source: arXiv:2105.11476 ancillary file (2021-05-24)
Supplement: Supplementary file 1 [file SI.pdf]

# Supplementary Information

*Random heterogeneity outperforms design in network synchronization*

Yuanzhao Zhang, Jorge L. Ocampo-Espindola, István Z. Kiss, and Adilson E. Motter

## SI TEXT

In the following sections, we present additional numerical and experimental results for generalizations of the oscillator networks considered in the main text.

**Systems with nonlinear coupling functions.** In the main text we focused on oscillators interacting through linear coupling functions. Here, we show that heterogeneity can also stabilize synchronization when the coupling function is nonlinear. As a representative example, we replace the linear coupling in Eq. 1 with sine coupling. The system is then described as

$$\dot{x}_j(t) = \lambda_j x_j(t) - \omega_j y_j(t) + \left(x_j^2(t) + y_j^2(t)\right)\left(\gamma_j y_j(t) - x_j(t)\right) + \frac{K}{d_j}\sum_{k=1}^{N} A_{jk} \sin\left(x_k(t-\tau) - x_j(t)\right), \tag{S1a}$$

$$\dot{y}_j(t) = \lambda_j y_j(t) + \omega_j x_j(t) - \left(x_j^2(t) + y_j^2(t)\right)\left(\gamma_j x_j(t) + y_j(t)\right) + \frac{K}{d_j}\sum_{k=1}^{N} A_{jk} \sin\left(y_k(t-\tau) - y_j(t)\right). \tag{S1b}$$

Using exactly the same parameters as in Fig. 1, we again observe the synchronizing effect of oscillator heterogeneity in our nonlinearly coupled system (Fig. S1).

**Systems with link-dependent coupling delays.** In the main text we considered systems with uniform coupling delays. Here, we show that the same phenomenon persists when the coupling delays are allowed to be heterogeneous, and each link can experience a different time delay. Such systems can be described by the following equation, which replaces the common coupling delay $\tau$ in Eq. 1 with link-specific delays $\tau_{jk}$ ($\tau_{jk}$ not necessarily equal to $\tau_{kj}$):

$$\dot{z}_j(t) = f_j(z_j(t)) + \frac{K}{d_j}\sum_{k=1}^{N} A_{jk}\left[z_k(t-\tau_{jk}) - z_j(t)\right]. \tag{S2}$$

Figure S2 shows results for the same system as in Fig. 1, except that the coupling delays are drawn from a Gaussian distribution with standard deviation 1 (the mean is still set to $1.8\pi$). These results confirm that oscillator heterogeneity can stabilize synchronization that is otherwise unstable even when the time delays vary from link to link.

**Random heterogeneity in all parameters.** In Fig. S3, we show that heterogeneity can also consistently induce synchronization when it is present in all three parameters of the oscillators. In this case, the parameters $\{\omega_j\}$, $\{\lambda_j\}$, and $r_0^2\{\gamma_j\}$ are all independently drawn from a Gaussian distribution with standard deviation $\sigma$.

**Effect of network size.** In Fig. S4, we explore how the network size affects the probability of inducing synchronization with random oscillator heterogeneity. In all cases the effect is persistent across a wide range of network sizes, for directed ring networks ranging from $N = 9$ to $N = 72$. It can be seen that the peak of the curve shifts leftward as $N$ increases, but it always maintains its height above 0.9 for all network sizes investigated here.

**Random heterogeneity in random networks and small-world networks.** Here, we show that random oscillator heterogeneity can also induce synchronization in networks beyond directed rings. In Fig. S5, two representative examples of random networks with common indegrees are studied in detail. The simulations show that random heterogeneity in any or all of the three parameters can consistently promote synchronization in both networks. Similar results are observed in Fig. S6 for a small-world network with heterogeneous degrees constructed by adding 20 random shortcuts to an 8-by-8 square lattice.

**Experiments on a small-world network.** In Fig. S7, we demonstrate experimentally that the same phenomenon can be observed in networks with heterogeneous degrees. As a representative example, we considered a small-world network formed by adding six random shortcuts to the 4-by-4 lattice used in Figs. 6 and 7 (Fig. S7*A*). The parameters used are similar to the ones reported in *Materials and Methods* for Figs. 6 and 7. Specifically, we set the coupling strength to $K = -0.25$ V/mA, the coupling delay to $\tau = 1.55$ s, and the circuit potential to $V_0 = 1.24$ V. The nominal oscillator heterogeneity was set to $\sigma = 0.13$ kohm in the heterogeneous system, while the mean resistance was fixed at 1.06 kohm for both homogeneous and heterogeneous systems.

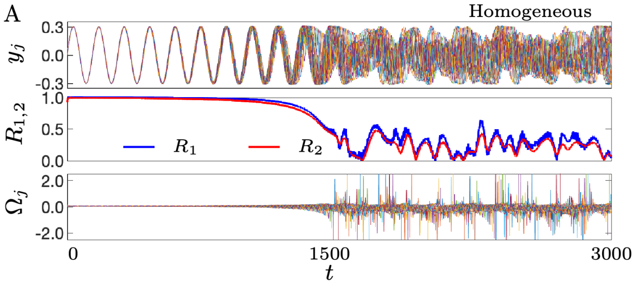


FIG. S1. Heterogeneity induces synchronization among Stuart-Landau oscillators with nonlinear coupling. All plotted quantities and parameters used are the same as in Fig. 1.

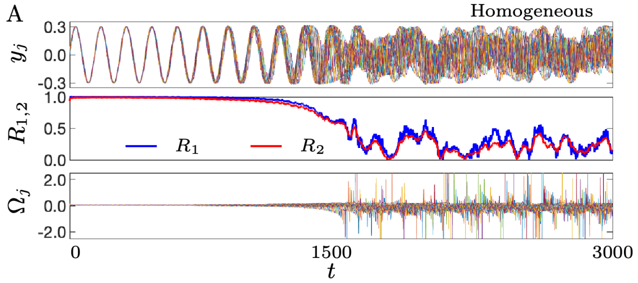


FIG. S2. Heterogeneity induces synchronization among Stuart-Landau oscillators with link-dependent coupling delays. All plotted quantities and parameters used are the same as in Fig. 1, with the exception of coupling delays, which have a mean of $1.8\pi$ and a standard deviation of 1.

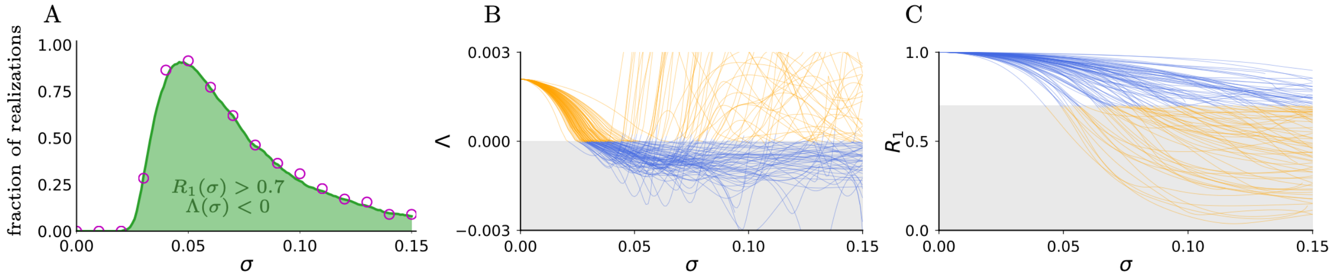


FIG. S3. Effect of random heterogeneity in all oscillator parameters. (*A*) Probability of inducing synchronization when heterogeneity is present in $\{\omega_j; \gamma_j; \lambda_j\}$, estimated from 1000 realizations of the heterogeneity profile. (*B*) MTLE $\Lambda(\sigma)$ for 100 such realizations, where the portions highlighted in blue correspond to $\Lambda(\sigma) < 0$. (*C*) Order parameter $R_1(\sigma)$ of the (possibly unstable) phase-locked state for the same 100 realizations, where blue indicates $R_1(\sigma) > 0.7$. The network and parameters are the same as in Fig. 3.

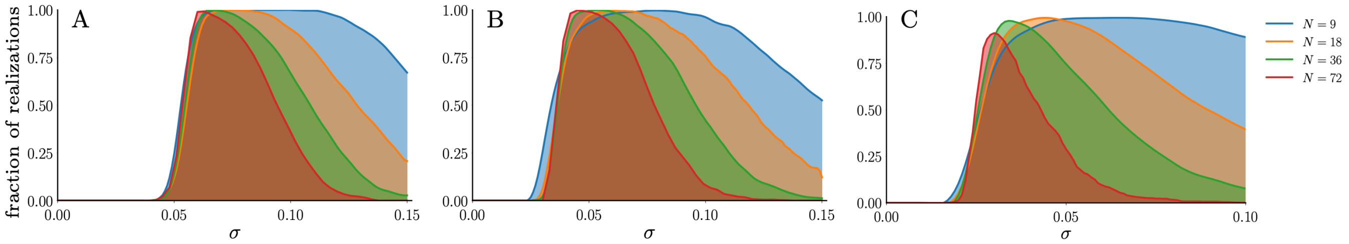


FIG. S4. Effect of random heterogeneity across network sizes. (*A*–*C*) Probability of inducing synchronization for heterogeneous $\{\omega_j\}$ (*A*), $\{\omega_j; \gamma_j\}$ (*B*), and $\{\omega_j; \gamma_j; \lambda_j\}$ (*C*) in directed ring networks of various sizes $N$. Each probability curve is estimated from 1000 realizations of the heterogeneity profile. The parameters are $\lambda = 0.1$, $\omega = 1.35$, $\gamma = 3.81$, $K = 0.3$, and $\tau = 1.8\pi$.

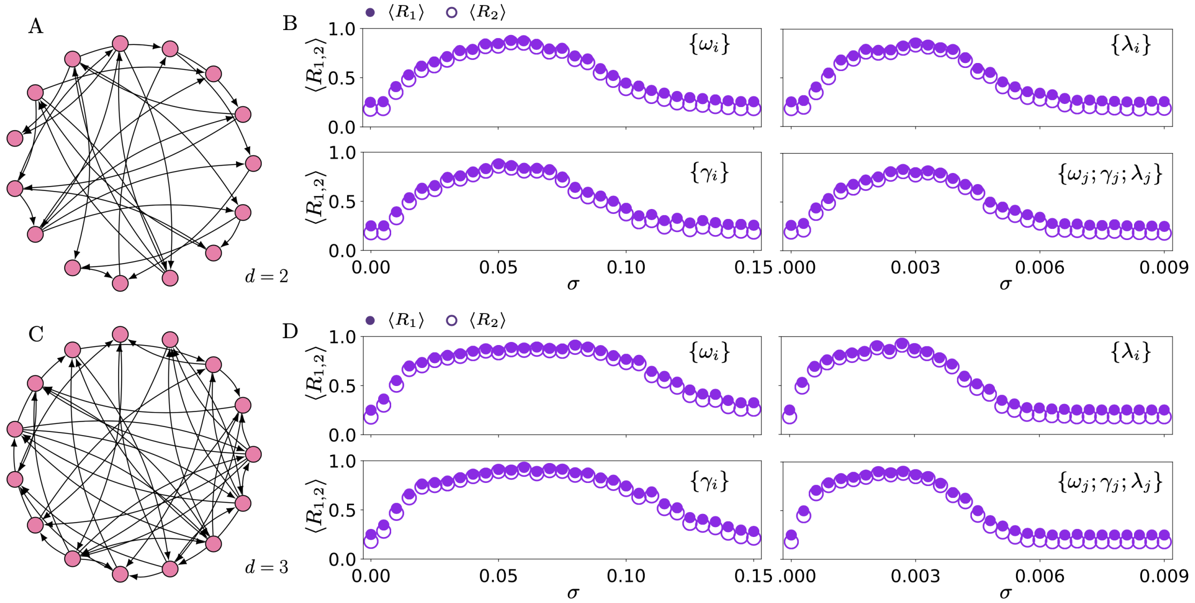


FIG. S5. Effect of random oscillator heterogeneity in random networks. ($A$) Random network with indegree $d = 2$. ($B$) Average order parameters for the network in $A$ with heterogeneity introduced in $\{\omega_j\}$, $\{\lambda_j\}$, $\{\gamma_j\}$, and $\{\omega_j; \gamma_j; \lambda_j\}$, respectively. ($C$) Random network with indegree $d = 3$. ($D$) Counterpart of $B$ for the network in $C$. The results in $B$ and $D$ are based on 300 realizations of the heterogeneity profile. The parameters for the homogeneous systems are chosen from the region where synchronization is unstable: $\lambda = 0.1$, $\omega = -2.7$, $\gamma = -30$, $K = 0.1$, and $\tau = 1.8\pi$ in $B$; $\lambda = 0.1$, $\omega = -3.9$, $\gamma = -42.8$, $K = 0.1$, and $\tau = 1.8\pi$ in $D$.

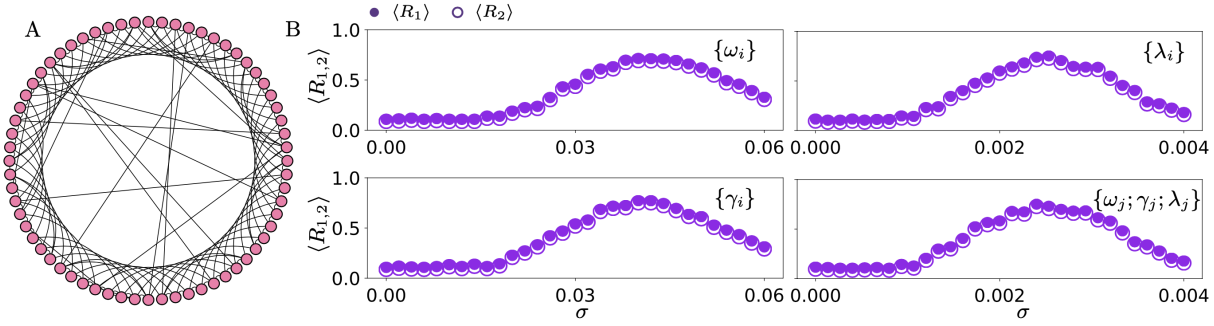


FIG. S6. Analog of Fig. S5 for a small-world network. ($A$) Small-world network with $N = 64$ nodes, obtained by adding 20 random shortcuts to an 8-by-8 lattice. ($B$) Average order parameters for the network in $A$ with heterogeneity introduced in $\{\omega_j\}$, $\{\lambda_j\}$, $\{\gamma_j\}$, and $\{\omega_j; \gamma_j; \lambda_j\}$, respectively. The parameters for the homogeneous system are chosen from the region where synchronization is unstable: $\lambda = 0.1$, $\omega = -2.4$, $\gamma = -26.7$, $K = 0.1$, and $\tau = 1.8\pi$.

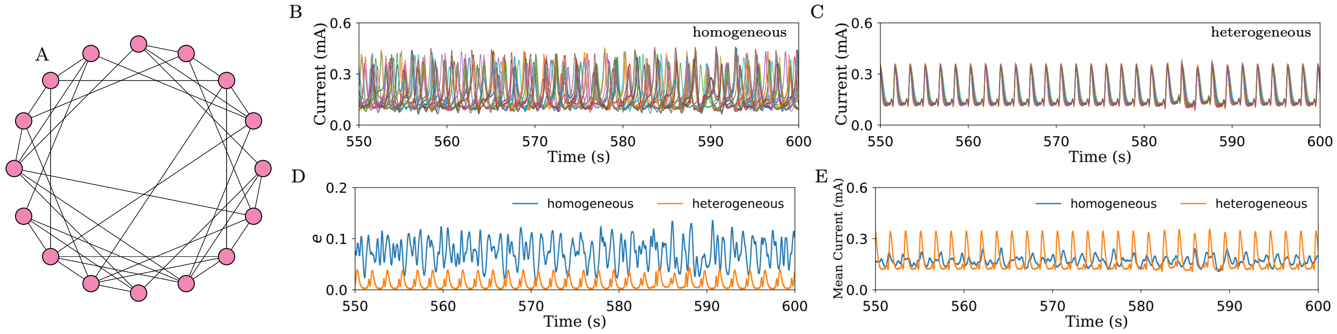


FIG. S7. Analog of Fig. 7 for experiments on a small-world network obtained by adding six random shortcuts to a 4-by-4 lattice. ($A$) Small-world network (with heterogeneous degrees) used in the electrochemical experiment. ($B$–$E$) We consistently observe desynchronization in the homogeneous system and robust synchronization in the heterogeneous system. The experimental parameters are set to $K = -0.25$ V/mA, $\tau = 1.55$ s, and $V_0 = 1.24$ V.

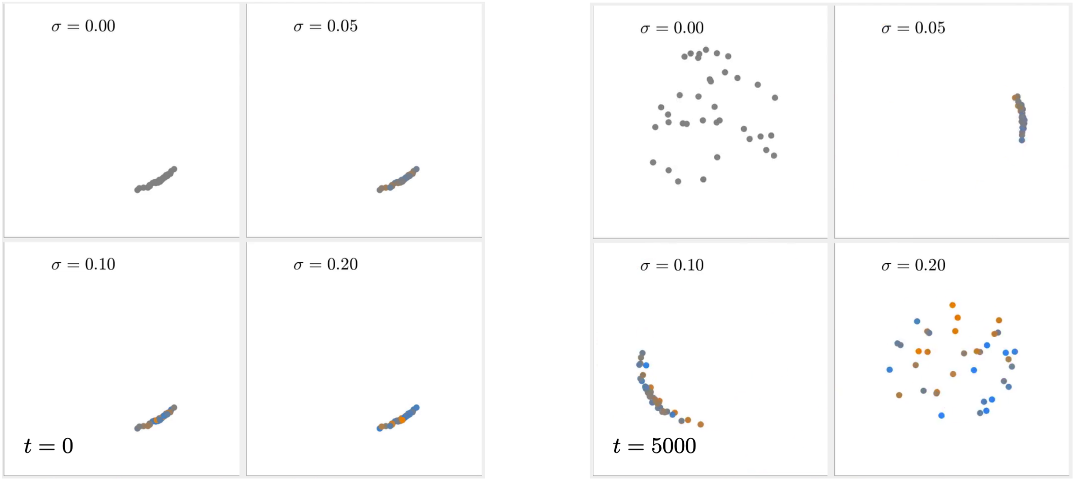


Movie S1. Animation showing the evolution of four systems of delay-coupled Stuart-Landau oscillators (snapshots shown above for two different times $t$). Each system consists of 36 oscillators (represented as dots moving in the complex plane), with different levels of random heterogeneity indicated by colors and quantified by $\sigma$. All four systems are initialized close to the identical synchronization state. After about 4000 time units, both systems on the diagonal (no heterogeneity and large heterogeneity) have evolved into an incoherent state, while the off-diagonal systems (intermediate heterogeneity) maintain a high level of synchronization, which persists indefinitely. The network structure is a directed ring and the parameters are the same as in Fig. 1.
